# Supplementary material for: Transverse Single Spin Asymmetries and Cross-Sections for Forward pi0 and eta Mesons at Large Feynman-x in sqrt(s)=200 GeV polarized p+p Collisions at STAR
Source: arXiv:1205.4771 source file (2012-05-21)
Supplement: Supplementary file 3 [file Dedication.tex]

To my wife Doeun, for her time independent love and support. \\
To our daughter Serina, for her life and joy.
