# Supplementary material for: Transverse Single Spin Asymmetries and Cross-Sections for Forward pi0 and eta Mesons at Large Feynman-x in sqrt(s)=200 GeV polarized p+p Collisions at STAR
Source: arXiv:1205.4771 source file (2012-05-21)
Supplement: Supplementary file 4 [file ListOfSymbols.tex]

% Place the list of symbols below.
\begin{eqlist}[\labelsep 1em]

\item[$\alpha$]
The first greek letter, p.~\pageref{}

\item[$\alpha$]
The first greek letter, p.~\pageref{}

\item[$\alpha$]
The first greek letter, but we should really add some more text, though we need it to go on two lines, p.~\pageref{}

\item[$\alpha$]
The first greek letter, p.~\pageref{}

\item[$\alpha$]
The first greek letter, p.~\pageref{}

\item[$\alpha$]
The first greek letter, p.~\pageref{}

\item[$\alpha$]
The first greek letter, p.~\pageref{}

\item[$\alpha$]
The first greek letter, p.~\pageref{}

\end{eqlist}
