# Supplementary material for: Transverse Single Spin Asymmetries and Cross-Sections for Forward pi0 and eta Mesons at Large Feynman-x in sqrt(s)=200 GeV polarized p+p Collisions at STAR
Source: arXiv:1205.4771 source file (2012-05-21)
Supplement: Supplementary file 5 [file Vita.tex]

% Place your vita below.

\begin{itemize}
\item Pennsylvania State University, PhD candidate in Physics, Aug, 2004 to present

\item Pennsylvania State University, B.S in Physics, May, 2004

\item Military Service, Korean Augmentation to the United States Army, Jan. 2001 to Mar. 2003

\item Seoul National University, English Literature Department, (no degree) Mar. 1996 to Dec. 1998

\item Myungduk Foreign Language High School, Seoul, Korea, HS Diploma, Mar. 1996 

\end{itemize}
